# Supplementary material for: Iron Intercalated Covalent-Organic Frameworks: First Crystalline Porous Thermoelectric Materials
Source: arXiv:1703.02613 source file (2017-03-07)
Supplement: Supplementary file 1 [file SI-COFs.pdf]

# Supporting Information

## Iron Intercalated Covalent-Organic Frameworks: First Crystalline Porous Thermoelectric Materials

Srimanta Pakhira[1,2], Kevin P. Lucht[1,2], Jose L. Mendoza-Cortes[1,2]

[1] Department of Chemical & Biomedical Engineering, FAMU-FSU Joint College of Engineering, and High Performance Materials Institute (HPMI), Florida State University, Tallahassee, Florida, 32310, USA.
[2] Condensed Matter Theory, National High Magnetic Field Laboratory (NHMFL), Scientific Computing Department, Materials Science and Engineering, Florida State University, Tallahassee, Florida, 32310, USA.

E-mail: mendoza@eng.famu.fsu.edu

# I. ALL THE .CIF STRUCTURES OF THE PRISTINE AND INTERCALATED-COFS

The optimized crystallographic information (.cif) files with optimized geometries have been provided below.

## A. COF-SU-00

```
data_BG_Triazine.out
_symmetry_space_group_name_H-M    'P-6M2'
_symmetry_Int_Tables_number       187
_symmetry_cell_setting            hexagonal
loop_
_symmetry_equiv_pos_as_xyz
  x,y,z
_cell_length_a                    14.7275
_cell_length_b                    14.7275
_cell_length_c                    3.2408
_cell_angle_alpha                 90.0000
_cell_angle_beta                  90.0000
_cell_angle_gamma                 120.0000
loop_
_atom_site_label
_atom_site_type_symbol
_atom_site_fract_x
_atom_site_fract_y
_atom_site_fract_z
_atom_site_U_iso_or_equiv
_atom_site_adp_type
_atom_site_occupancy
C001   C    -0.38821  -0.44832   0.00000   0.00000  Uiso   1.00
C007   C     0.04784  -0.39468  -0.00000   0.00000  Uiso   1.00
H013   H     0.40727   0.10371  -0.00000   0.00000  Uiso   1.00
H019   H    -0.40041  -0.30980   0.00000   0.00000  Uiso   1.00
C025   C    -0.38476   0.38476  -0.00000   0.00000  Uiso   1.00
C028   C    -0.44247   0.44247   0.00000   0.00000  Uiso   1.00
B031   B     0.38811  -0.38811  -0.00000   0.00000  Uiso   1.00
N034   N    -0.27996   0.27996  -0.00000   0.00000  Uiso   1.00
C037   C     0.44818  -0.44818  -0.00000   0.00000  Uiso   1.00
O040   O     0.27968  -0.27968   0.00000   0.00000  Uiso   1.00
```

## B. COF-SU-01

```
data_BG_Fe3_triazine.out
_symmetry_space_group_name_H-M    'P-6M2'
_symmetry_Int_Tables_number       187
_symmetry_cell_setting            hexagonal
loop_
_symmetry_equiv_pos_as_xyz
  x,y,z
_cell_length_a                    14.8311
_cell_length_b                    14.8311
_cell_length_c                    3.4436
_cell_angle_alpha                 90.0000
_cell_angle_beta                  90.0000
_cell_angle_gamma                 120.0000
loop_
_atom_site_label
_atom_site_type_symbol
_atom_site_fract_x
_atom_site_fract_y
_atom_site_fract_z
_atom_site_U_iso_or_equiv
_atom_site_adp_type
_atom_site_occupancy
C001   C    -0.38597  -0.44685   0.00000   0.00000  Uiso   1.00
C007   C     0.04847  -0.39240   0.00000   0.00000  Uiso   1.00
H013   H     0.40659   0.10439  -0.00000   0.00000  Uiso   1.00
H019   H    -0.39936  -0.30842   0.00000   0.00000  Uiso   1.00
C025   C    -0.38441   0.38441  -0.00000   0.00000  Uiso   1.00
C028   C    -0.44073   0.44073  -0.00000   0.00000  Uiso   1.00
B031   B     0.38771  -0.38771   0.00000   0.00000  Uiso   1.00
N034   N    -0.28000   0.28000  -0.00000   0.00000  Uiso   1.00
C037   C     0.44649  -0.44649   0.00000   0.00000  Uiso   1.00
O040   O     0.27983  -0.27983   0.00000   0.00000  Uiso   1.00
FE043  Fe   -0.49763   0.49763  -0.50000   0.00000  Uiso   1.00
```

## C. COF-SU-02

```
data_BG_Fe4_triazine.out
_symmetry_space_group_name_H-M    'P-6M2'
```

```
_symmetry_Int_Tables_number       187
_symmetry_cell_setting            hexagonal
loop_
_symmetry_equiv_pos_as_xyz
  x,y,z
_cell_length_a                    14.9482
_cell_length_b                    14.9482
_cell_length_c                    3.4482
_cell_angle_alpha                 90.0000
_cell_angle_beta                  90.0000
_cell_angle_gamma                 120.0000
loop_
_atom_site_label
_atom_site_type_symbol
_atom_site_fract_x
_atom_site_fract_y
_atom_site_fract_z
_atom_site_U_iso_or_equiv
_atom_site_adp_type
_atom_site_occupancy
C001   C    -0.38561  -0.44844   0.00000   0.00000  Uiso   1.00
C007   C     0.04584  -0.39468   0.00000   0.00000  Uiso   1.00
H013   H     0.40834   0.10584  -0.00000   0.00000  Uiso   1.00
H019   H    -0.39919  -0.31132   0.00000   0.00000  Uiso   1.00
C025   C    -0.38400   0.38400  -0.00000   0.00000  Uiso   1.00
C028   C    -0.43988   0.43988  -0.00000   0.00000  Uiso   1.00
B031   B     0.39010  -0.39010  -0.00000   0.00000  Uiso   1.00
N034   N    -0.28041   0.28041   0.00000   0.00000  Uiso   1.00
C037   C     0.44820  -0.44820  -0.00000   0.00000  Uiso   1.00
O040   O     0.27953  -0.27953   0.00000   0.00000  Uiso   1.00
FE043  Fe   -0.49468   0.49468  -0.50000   0.00000  Uiso   1.00
FE046  Fe    0.33333  -0.33333  -0.50000   0.00000  Uiso   1.00
```

### D. COF-SU-03

```
data_BG_Fe5_triazine.out
_symmetry_space_group_name_H-M    'P-6M2'
_symmetry_Int_Tables_number       187
_symmetry_cell_setting            hexagonal
loop_
_symmetry_equiv_pos_as_xyz
  x,y,z
_cell_length_a                    15.0303
_cell_length_b                    15.0303
_cell_length_c                    3.4398
_cell_angle_alpha                 90.0000
_cell_angle_beta                  90.0000
_cell_angle_gamma                 120.0000
loop_
_atom_site_label
_atom_site_type_symbol
_atom_site_fract_x
_atom_site_fract_y
_atom_site_fract_z
_atom_site_U_iso_or_equiv
_atom_site_adp_type
_atom_site_occupancy
C001   C    -0.38724  -0.44830   0.00000   0.00000  Uiso   1.00
C007   C     0.04713  -0.39421   0.00000   0.00000  Uiso   1.00
H013   H     0.40853   0.10397  -0.00000   0.00000  Uiso   1.00
H019   H    -0.40016  -0.31134   0.00000   0.00000  Uiso   1.00
C025   C    -0.38578   0.38578  -0.00000   0.00000  Uiso   1.00
C028   C    -0.44123   0.44123  -0.00000   0.00000  Uiso   1.00
B031   B     0.38976  -0.38976   0.00000   0.00000  Uiso   1.00
N034   N    -0.27898   0.27898  -0.00000   0.00000  Uiso   1.00
C037   C     0.44767  -0.44767   0.00000   0.00000  Uiso   1.00
O040   O     0.27980  -0.27980   0.00000   0.00000  Uiso   1.00
FE043  Fe   -0.49787   0.49787  -0.50000   0.00000  Uiso   1.00
FE046  Fe    0.33333  -0.33333  -0.50000   0.00000  Uiso   1.00
FE047  Fe   -0.33333   0.33333  -0.50000   0.00000  Uiso   1.00
```
